# Supplementary material for: PhoneMD: Learning to Diagnose Parkinson's Disease from Smartphone Data
Source: arXiv:1810.01485 source file (2018-11-14)
Supplement: Supplementary file 1 [file appendix.pdf]

# Supplementary Material for:
# "Learning to Diagnose Parkinson's Disease from Smartphone Data"

**Patrick Schwab**
Institute of Robotics and Intelligent Systems
ETH Zurich, Switzerland
patrick.schwab@hest.ethz.ch

**Walter Karlen**
Institute of Robotics and Intelligent Systems
ETH Zurich, Switzerland
walter.karlen@hest.ethz.ch

## Appendix A. Random Forest Features

The features used in the random forest (RF) models are listed in Tables S1, S2, S3, and S4. We chose our features based on prior research (Arora et al. 2015). We did not use all features reported in (Arora et al. 2015) because some of those features were too computationally inefficient to run in a reasonable amount of time in a dataset of the given size.

## Appendix B. Neural Network Architectures

**Walking Test.** For the walking test, we used a convolutional neural network (CNN) with temporal convolutions, a kernel size of 3, a number of sequential hidden layers, and an initial number of neurons with a growth rate per additional convolutional layer of 8. The number of initial neurons and the number of hidden layers were hyperparameters chosen at random from the ranges listed in Appendix C. The convolutional layers were followed by an attention mechanism as described in the main body of the paper, a single fully-connected layer with 32 neurons and an output neuron with a sigmoid activation. All layers except the output layer were followed by a batch normalisation layer and a leaky ReLU activation with a negative slope coefficient $\alpha$ of 0.3.

**Voice Test.** For the voice test, we used a CNN with spatial convolutions, a kernel size of 3, a number of sequential hidden layers, and an initial number of neurons with a growth rate per additional convolutional layer of 8. The number of initial neurons and the number of hidden layers were hyperparameters chosen at random from the ranges listed in Appendix C. The convolutional layers were by three fully-connected layers with 512, 256 and 32 neurons, respectively, and an output neuron with a sigmoid activation. All layers except the output layer were followed by a batch normalisation layer and a leaky ReLU activation with a negative slope coefficient $\alpha$ of 0.3.

**Tapping Test.** For the tapping test, we used a recurrent neural network (RNN) for the tapping inputs with one bidirectional long short-term memory (BLSTM) layer, and a number of neurons for the BLSTM layer. The number of neurons for the BLSTM layer was a hyperparameter chosen at random from the range listed in Appendix C. The recurrent layer was followed by an attention mechanism as described in the main body of the paper. All layers except the output layer were followed by a batch normalisation layer. In addition to the RNN for the tapping inputs, we used a CNN to jointly process the accelerometer signal. For the accelerometer neural network, we used a CNN with temporal convolutions, a kernel size of 3, a number of sequential hidden layers, and an initial number of neurons with a growth rate per additional convolutional layer of 4. The number of initial neurons and the number of hidden layers were hyperparameters chosen at random from the ranges listed in Appendix C. The convolutional layers were followed by a single fully-connected layer with 32 neurons that was concatenated with the output of the RNN and then fed to an output neuron with a sigmoid activation.

Copyright © 2019, Association for the Advancement of Artificial Intelligence (www.aaai.org). All rights reserved.

**Memory Test.** For the memory test, we used a RNN with number of BLSTM layers, and a number of neurons for the BLSTM layers. The number of BLSTM layers and the number of neurons for the BLSTM layers were hyperparameters chosen at random from the ranges listed in Appendix C. The recurrent layers were followed by an attention mechanism as described in the main body of the paper. All layers except the output layer were followed by a batch normalisation layer.

**Evidence Aggregation Model (EAM).** For the EAM, we used a RNN with a number of BLSTM layers, and a number of neurons for the BLSTM layer. The number of BLSTM layers and the number of neurons for the BLSTM layers were hyperparameters chosen at random from the ranges listed in Appendix C. The recurrent layers were followed by an attention mechanism as described in the main body of the paper, and an output neuron with a sigmoid activation. All layers except the output layer were followed by a batch normalisation layer.

## Appendix C. Hyperparameters

**RF Hyperparameters.** For the RF models, we varied the number of trees between 512 to 1024 and the maximum depth of trees within the forest between 2 and 5.

**Neural Network Hyperparameters.** For the neural network models, we varied the dropout percentage after each hidden layer between 0 and 70%, and the L2 weight penalty from (0.0, 0.0001, 0.00001). For the EAMs, we varied the number of neurons per hidden layer between 16 to 64 and the number of hidden layers between 1 and 3. We also used different hyperparameter ranges for the specialised predictive models of each test type. For the walking test, we varied the number of neurons per hidden layer between 8 to 72 and the number of hidden layers between 5 and 7. For the voice test, we varied the number of neurons per hidden layer between 8 to 72 and the number of hidden layers between 5 and 6. For the tapping test, we varied the number of neurons per hidden layer between 8 to 64 and the number of hidden layers between 6 and 8. For the memory test, we varied the number of neurons per hidden layer between 8 to 72 and the number of hidden layers between 1 and 2. We varied the numbers of hidden layers covered by the hyperparameter search depending on which type of neural network was used for the test (CNN or RNN), and depending on the total sequence length of the test's input signals.

## Appendix D. Per-test Population Statistics

The population statistics of the dataset folds used to train the specialised predictive models for each test type differed significantly (Tables S5, S6, S7, and S8). We split the subjects along the same folds as in the experiments for the aggregated models in order to prevent information leakage when training the specialised predictive models. This led to the evaluated folds for each test type being significantly different, as not all subjects in the per-test subsets performed at least one test of a given type, and, for some tests, different user groups (PD or control) preferred to do tests in different amounts. For example, the ratio of test set samples done by people with PD varies from 66% for the tapping test to 88% for the memory test. A direct comparison of the relative performances of the specialised predictive models between test types was therefore not possible, since the evaluation metrics are influenced not just by the performance differences between predictive models but also by the different underlying population statistics.

## Appendix E. Memory and Tapping Samples

We present typical samples of attention distributions for memory and tapping tasks in Figures S1 and S2, respectively.

Table S1: Features used as inputs to the random forests (RFs) used to assess walking tests. The features were calculated on both the x and z channel of the accelerometer data. The RF models did not use the gyroscope data.

| walking | |
|---|---|
| Feature | Reference / Brief description |
| Mean | The mean of the amplitude of the input signal. |
| Standard deviation | The standard deviation of the amplitude of the input signal. |
| 25% quartile | The 25% quartile of the amplitude of the input signal. |
| 75% quartile | The 75% quartile of the amplitude of the input signal. |
| Inter-quartile range | The inter-quartile range of the amplitude of the input signal. |
| Median | The median of the amplitude of the input signal. |
| Range | The total range (max - min) of values of the input signal. |
| Skewness | The skewness of the amplitude of the input signal. |
| Kurtosis | The kurtosis of the amplitude of the input signal. |
| Mean squared energy | The mean squared energy of the amplitude of the input signal. |
| Entropy | The entropy of the input signal. |
| Mutual information | The mutual information of the input signal with the y-axis signal. |
| Detrended fluctuation analysis | (Arora et al. 2015) |
| Mean Teager-Kaiser energy operator | (Arora et al. 2015) |
| Cross-correlation | The cross-correlation of the input signal with itself up to lag level 1. |
| Zero-crossing rate | The zero-crossing rate of the input signal. |

Table S2: Features used as inputs to the RFs used to assess voice tests. The features were calculated on the raw audio signal of the voice test. The RF models did not use the recordings taken during the countdown leading up to the voice test.

| voice | |
|---|---|
| Feature | Reference / Brief description |
| Detrended fluctuation analysis | (Arora et al. 2015) |
| Mean Teager-Kaiser energy operator | (Arora et al. 2015) |
| Jitter | (Arora et al. 2015) |
| Shimmer | (Arora et al. 2015) |
| Pitch period entropy | (Arora et al. 2015) |
| Mel-frequency cepstral coefficients | (Arora et al. 2015) |

Table S3: Features used as inputs to the RFs used to assess tapping tests. The features were calculated on the inter-tap intervals and tap positions.

| tapping | |
|---|---|
| Feature | Reference / Brief description |
| Standard deviation | The standard deviation of the amplitude of the input signal. |
| Mean squared energy | The mean squared energy of the amplitude of the input signal. |
| Mean Teager-Kaiser energy operator | (Arora et al. 2015) |
| Cross-correlation | The cross-correlation of the input signal with itself up to lag level 2. |
| Detrended fluctuation analysis | (Arora et al. 2015) |
| $\text{Fatigue}_{10\%}$ | (Arora et al. 2015) |
| $\text{Fatigue}_{25\%}$ | (Arora et al. 2015) |
| $\text{Fatigue}_{50\%}$ | (Arora et al. 2015) |
| Tremor between taps | (Arora et al. 2015) |
| Finger opening angle | (Arora et al. 2015) |

Table S4: Features used as inputs to the RFs used to assess tapping tests. The features were calculated on the inter-tap intervals and the button hit/miss time series. We additionally used the meta data associated with the memory test (overall score, number of games played, number of failures).

| | memory |
|---|---|
| Feature | Reference / Brief description |
| Mean | The mean of the amplitude of the input signal. |
| Standard deviation | The standard deviation of the amplitude of the input signal. |
| Mean squared energy | The mean squared energy of the amplitude of the input signal. |
| Mean Teager-Kaiser energy operator | (Arora et al. 2015) |
| Cross-correlation | The cross-correlation of the input signal with itself up to lag level 2. |
| Detrended fluctuation analysis | (Arora et al. 2015) |
| Memory meta-data | The meta-data of the memory test. |
| $\text{Fatigue}_{10\%}$ | (Arora et al. 2015) |
| $\text{Fatigue}_{25\%}$ | (Arora et al. 2015) |
| $\text{Fatigue}_{50\%}$ | (Arora et al. 2015) |

Table S5: Population statistics of the training, validation, and test set for the walking tests. Numbers (#) shown are either absolute (Samples, Subjects), or mean ± standard deviation over all subjects.

| Property | Training | Validation | Test |
|---|---|---|---|
| Samples (#) | 8461 | 1496 | 2119 |
| PD (Samples, %) | 57.94 | 59.09 | 68.19 |
| Subjects (#) | 609 (71%) | 96 (11%) | 151 (18%) |
| PD (Subjects, %) | 43.19 | 44.79 | 47.68 |
| Female (%) | 26.77 | 34.38 | 19.21 |
| Age (years) | 59.71 ± 9.14 | 60.57 ± 8.56 | 58.62 ± 8.94 |
| Usage (days) | 31.08 ± 44.94 | 38.67 ± 51.52 | 32.50 ± 47.84 |

Table S6: Population statistics of the training, validation, and test set for the voice tests. Numbers (#) shown are either absolute (Samples, Subjects), or mean ± standard deviation over all subjects.

| Property | Training | Validation | Test |
|---|---|---|---|
| Samples (#) | 14176 | 2745 | 3586 |
| PD (Samples, %) | 54.36 | 49.25 | 69.77 |
| Subjects (#) | 880 (70%) | 141 (11%) | 241 (19%) |
| PD (Subjects, %) | 45.00 | 47.51 | 49.79 |
| Female (%) | 28.64 | 38.30 | 27.80 |
| Age (years) | 59.28 ± 9.29 | 59.65 ± 8.69 | 58.75 ± 9.36 |
| Usage (days) | 28.48 ± 43.72 | 33.42 ± 47.29 | 28.07 ± 44.88 |

Table S7: Population statistics of the training, validation, and test set for the tapping tests. Numbers (#) shown are either absolute (Samples, Subjects), or mean ± standard deviation over all subjects.

| Property | Training | Validation | Test |
|---|---|---|---|
| Samples (#) | 15823 | 2923 | 4064 |
| PD (Samples, %) | 51.85 | 48.58 | 66.63 |
| Subjects (#) | 1041 (70%) | 158 (11%) | 275 (19%) |
| PD (Subjects, %) | 42.84 | 42.41 | 48.00 |
| Female (%) | 28.05 | 37.34 | 27.27 |
| Age (years) | 58.59 ± 9.30 | 58.94 ± 8.75 | 58.35 ± 9.19 |
| Usage (days) | 25.16 ± 41.56 | 30.23 ± 45.83 | 26.48 ± 43.78 |

Table S8: Population statistics of the training, validation, and test set for the memory tests. We included memory tests done on medication, because there were few tests done off medication. Numbers (#) shown are either absolute (Samples, Subjects), or mean $\pm$ standard deviation over all subjects.

| Property | Training | Validation | Test |
|---|---|---|---|
| Samples (#) | 4720 | 1143 | 1600 |
| PD (Samples, %) | 88.62 | 86.18 | 87.81 |
| Subjects (#) | 337 (70%) | 55 (11%) | 91 (19%) |
| PD (Subjects, %) | 64.09 | 65.45 | 75.82 |
| Female (%) | 35.01 | 27.27 | 28.57 |
| Age (years) | 61.11 $\pm$ 9.05 | 61.29 $\pm$ 7.91 | 61.93 $\pm$ 8.87 |
| Usage (days) | 56.34 $\pm$ 57.19 | 66.10 $\pm$ 57.22 | 59.32 $\pm$ 60.65 |

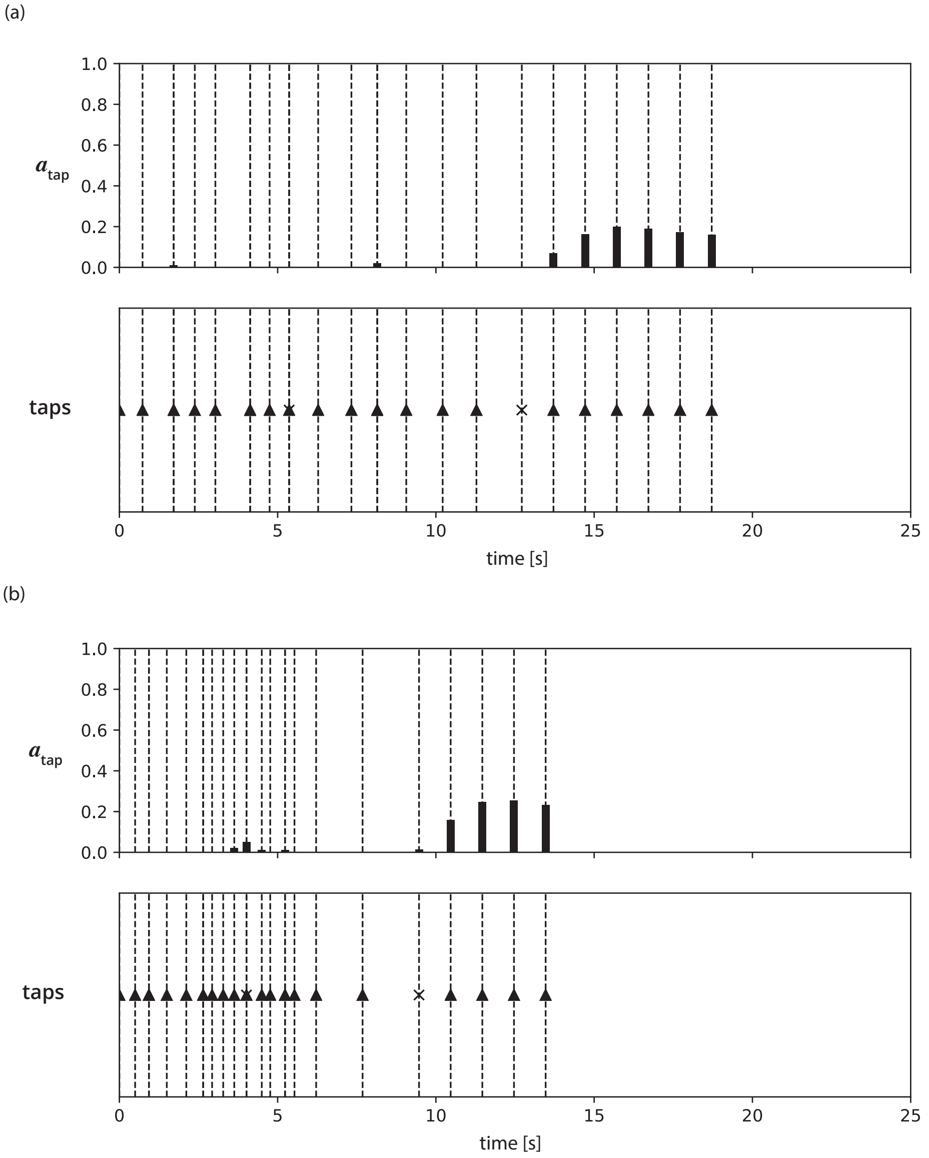


Figure S1: The outputs of the per-test neural attention mechanism ($a_{\text{tap}}$, top) on two representative samples (triangles and crosses, bottom) of memory tests from a user with Parkinson's disease. Triangles indicate correctly identified sequence elements and crosses indicate mistakes. We found that the predictive model's attention was typically focused on the more difficult final stage of the game. This pattern is visible in both samples (a) and (b). In both samples, we found that even mistakes in the early stage of the game do not receive a lot of attention relative to the more difficult end stage of the game.

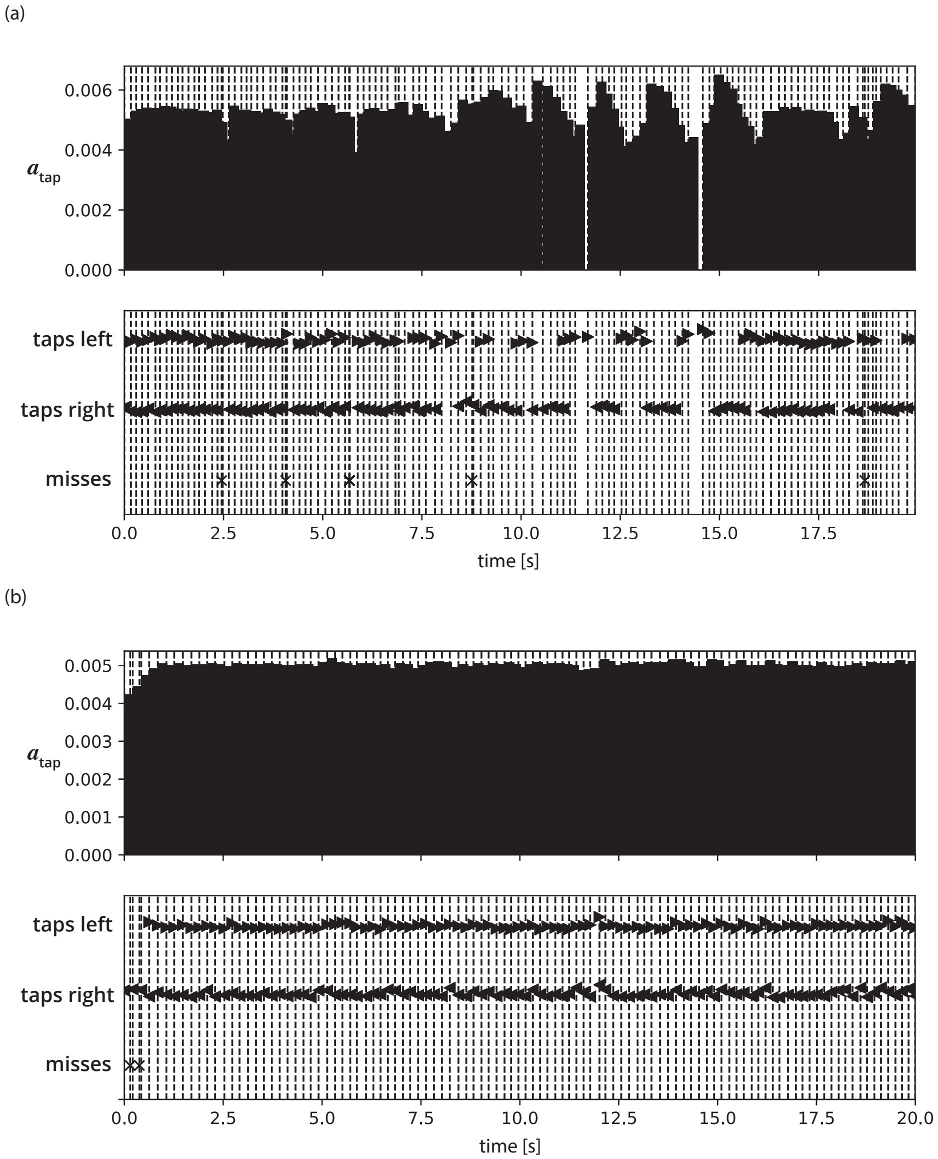


Figure S2: The outputs of the per-test neural attention mechanism ($a_{\text{tap}}$, top) on two representative samples (triangles and crosses, bottom) of tapping tests from a user with Parkinson's disease. The displacement of the tap triangles indicates the distance from the respective button's centre coordinate. In sample (a), we found that the assigned attention was typically lower in regions where the test was not performed properly (large breaks between taps, taps only on one side) and when taps were outside of the buttons' hit boxes (misses). In sample (b), we saw an almost uniform attention distribution, likely owing to the fact that the test was performed cleanly (aside from two misses at the start of the test). Our findings indicate that mistakes made in this test were not seen as predictive of Parkinson's disease. The predictive model instead focused on the user's overall tapping performance when the test was performed as intended. Furthermore, the predictive model distributed its attention among large numbers of taps, indicating that features spanning over many taps were in general seen as more predictive than individual taps.
